# Supplementary material for: Observation of azimuth-dependent suppression of hadron pairs in electron scattering off nuclei
Source: arXiv:2207.06682 source file (2022-11-05)
Supplement: Supplementary file 1 [file appendix1.tex]

\section*{Supplemental Material} \label{sec:appendix}
The values of $R_{2h}$, shown in Fig.~\ref{fig:R2withHERMES},  are listed in Tables~\ref{tab:z2_data}, \ref{tab:dphi_data}, and \ref{tab:mass_data}, along with the edges of the bins, and the statistical and systematic uncertainties.

\begin{table*}[h]
    \centering
    \caption{Values of $R_{2h}$ obtained for each target and each $z_2$ bin $\pm$ the statistical uncertainty for each data point $\pm$ the systematic uncertainty for each data point.  These data correspond to those shown in Fig.~\ref{fig:R2withHERMES}(a)}
    \setlength{\tabcolsep}{12pt}
    \label{tab:z2_data}
    \begin{tabular}{c|c|c|c}
         $z_2$ & $R_{2h}$(C, $z_2$) & $R_{2h}$(Fe, $z_2$) & $R_{2h}$(Pb, $z_2$)\\
         \hline
0.05--0.10 & 0.982$\pm$0.017$\pm$0.036 & 0.917$\pm$0.015$\pm$0.034 & 0.824$\pm$0.020$\pm$0.030\\
0.10--0.15 & 0.819$\pm$0.010$\pm$0.026 & 0.732$\pm$0.008$\pm$0.024 & 0.696$\pm$0.013$\pm$0.022\\
0.15--0.20 & 0.823$\pm$0.014$\pm$0.021 & 0.724$\pm$0.011$\pm$0.019 & 0.694$\pm$0.017$\pm$0.018\\
0.20--0.25 & 0.870$\pm$0.018$\pm$0.023 & 0.757$\pm$0.014$\pm$0.020 & 0.700$\pm$0.021$\pm$0.018\\
0.25--0.30 & 0.840$\pm$0.022$\pm$0.022 & 0.752$\pm$0.018$\pm$0.020 & 0.702$\pm$0.026$\pm$0.019\\
0.30--0.35 & 0.941$\pm$0.035$\pm$0.027 & 0.769$\pm$0.026$\pm$0.022 & 0.713$\pm$0.038$\pm$0.021\\
0.35--0.40 & 0.911$\pm$0.050$\pm$0.033 & 0.749$\pm$0.036$\pm$0.027 & 0.712$\pm$0.057$\pm$0.026\\
0.40--0.45 & 1.163$\pm$0.108$\pm$0.049 & 0.955$\pm$0.074$\pm$0.040 & 0.934$\pm$0.112$\pm$0.039\\
    \end{tabular}
\end{table*}

\begin{table*}[h]
    \centering
    \caption{Values of $R_{2h}$ obtained for each target and each $|\Delta\phi|$ bin $\pm$ the statistical uncertainty for each data point $\pm$ the systematic uncertainty for each data point.  These data correspond to those shown in Fig.~\ref{fig:R2withHERMES}(b)}
    \setlength{\tabcolsep}{12pt}
    \label{tab:dphi_data}
    \begin{tabular}{c|c|c|c}
$|\Delta\phi|$ [rad]& $R_{2h}$(C, $|\Delta\phi|$) & $R_{2h}$(Fe, $|\Delta\phi|$) & $R_{2h}$(Pb, $|\Delta\phi|$)\\
\hline
0.00--0.39 & 1.019$\pm$0.031$\pm$0.043 & 0.968$\pm$0.026$\pm$0.041 & 0.944$\pm$0.039$\pm$0.035\\
0.39--0.79 & 0.962$\pm$0.028$\pm$0.030 & 0.908$\pm$0.023$\pm$0.029 & 0.878$\pm$0.035$\pm$0.028\\
0.79--1.18 & 0.976$\pm$0.027$\pm$0.026 & 0.895$\pm$0.021$\pm$0.023 & 0.878$\pm$0.033$\pm$0.023\\
1.18--1.57 & 0.944$\pm$0.022$\pm$0.024 & 0.890$\pm$0.018$\pm$0.022 & 0.827$\pm$0.026$\pm$0.021\\
1.57--1.96 & 0.876$\pm$0.018$\pm$0.022 & 0.775$\pm$0.014$\pm$0.020 & 0.802$\pm$0.023$\pm$0.021\\
1.96--2.35 & 0.841$\pm$0.016$\pm$0.021 & 0.724$\pm$0.012$\pm$0.018 & 0.675$\pm$0.018$\pm$0.020\\
2.35--2.75 & 0.812$\pm$0.014$\pm$0.021 & 0.705$\pm$0.011$\pm$0.019 & 0.611$\pm$0.015$\pm$0.022\\
2.75--3.14 & 0.789$\pm$0.013$\pm$0.024 & 0.671$\pm$0.010$\pm$0.020 & 0.620$\pm$0.015$\pm$0.026\\
    \end{tabular}
\end{table*}

\begin{table*}[h]
    \centering
    \caption{Values of $R_{2h}$ obtained for each target and each $m_{\pi\pi}$ bin $\pm$ the statistical uncertainty for each data point $\pm$ the systematic uncertainty for each data point.  These data correspond to those shown in Fig.~\ref{fig:R2withHERMES}(c)}
    \setlength{\tabcolsep}{12pt}
    \label{tab:mass_data}
    \begin{tabular}{c|c|c|c}
$m_{\pi\pi}$ [GeV] & $R_{2h}$(C, $m_{\pi\pi}$) & $R_{2h}$(Fe, $m_{\pi\pi}$) & $R_{2h}$(Pb, $m_{\pi\pi}$)\\
\hline
0.30--0.44 & 1.021$\pm$0.057$\pm$0.035 & 0.914$\pm$0.041$\pm$0.031 & 0.836$\pm$0.066$\pm$0.030\\
0.44--0.58 & 0.962$\pm$0.030$\pm$0.046 & 0.896$\pm$0.023$\pm$0.043 & 0.874$\pm$0.037$\pm$0.042\\
0.58--0.72 & 0.920$\pm$0.019$\pm$0.023 & 0.813$\pm$0.015$\pm$0.021 & 0.798$\pm$0.023$\pm$0.020\\
0.72--0.86 & 0.878$\pm$0.013$\pm$0.023 & 0.782$\pm$0.010$\pm$0.020 & 0.782$\pm$0.016$\pm$0.020\\
0.86--1.00 & 0.831$\pm$0.014$\pm$0.023 & 0.721$\pm$0.011$\pm$0.020 & 0.670$\pm$0.016$\pm$0.018\\
1.00--1.14 & 0.769$\pm$0.015$\pm$0.021 & 0.685$\pm$0.012$\pm$0.019 & 0.604$\pm$0.017$\pm$0.017\\
1.14--1.28 & 0.834$\pm$0.018$\pm$0.026 & 0.725$\pm$0.015$\pm$0.023 & 0.647$\pm$0.021$\pm$0.020\\
1.28--1.42 & 0.913$\pm$0.028$\pm$0.035 & 0.782$\pm$0.023$\pm$0.030 & 0.734$\pm$0.033$\pm$0.028\\
1.42--1.56 & 0.952$\pm$0.049$\pm$0.046 & 0.913$\pm$0.043$\pm$0.044 & 0.716$\pm$0.054$\pm$0.041\\
1.56--1.70 & 1.410$\pm$0.116$\pm$0.095 & 1.173$\pm$0.089$\pm$0.079 & 1.092$\pm$0.124$\pm$0.094\\
 \end{tabular}
\end{table*}
